# Supplementary material for: UAV Formation and Resource Allocation Optimization for Communication-Assisted 3D InSAR Sensing
Source: arXiv:2407.06607 source file (2025-02-07)

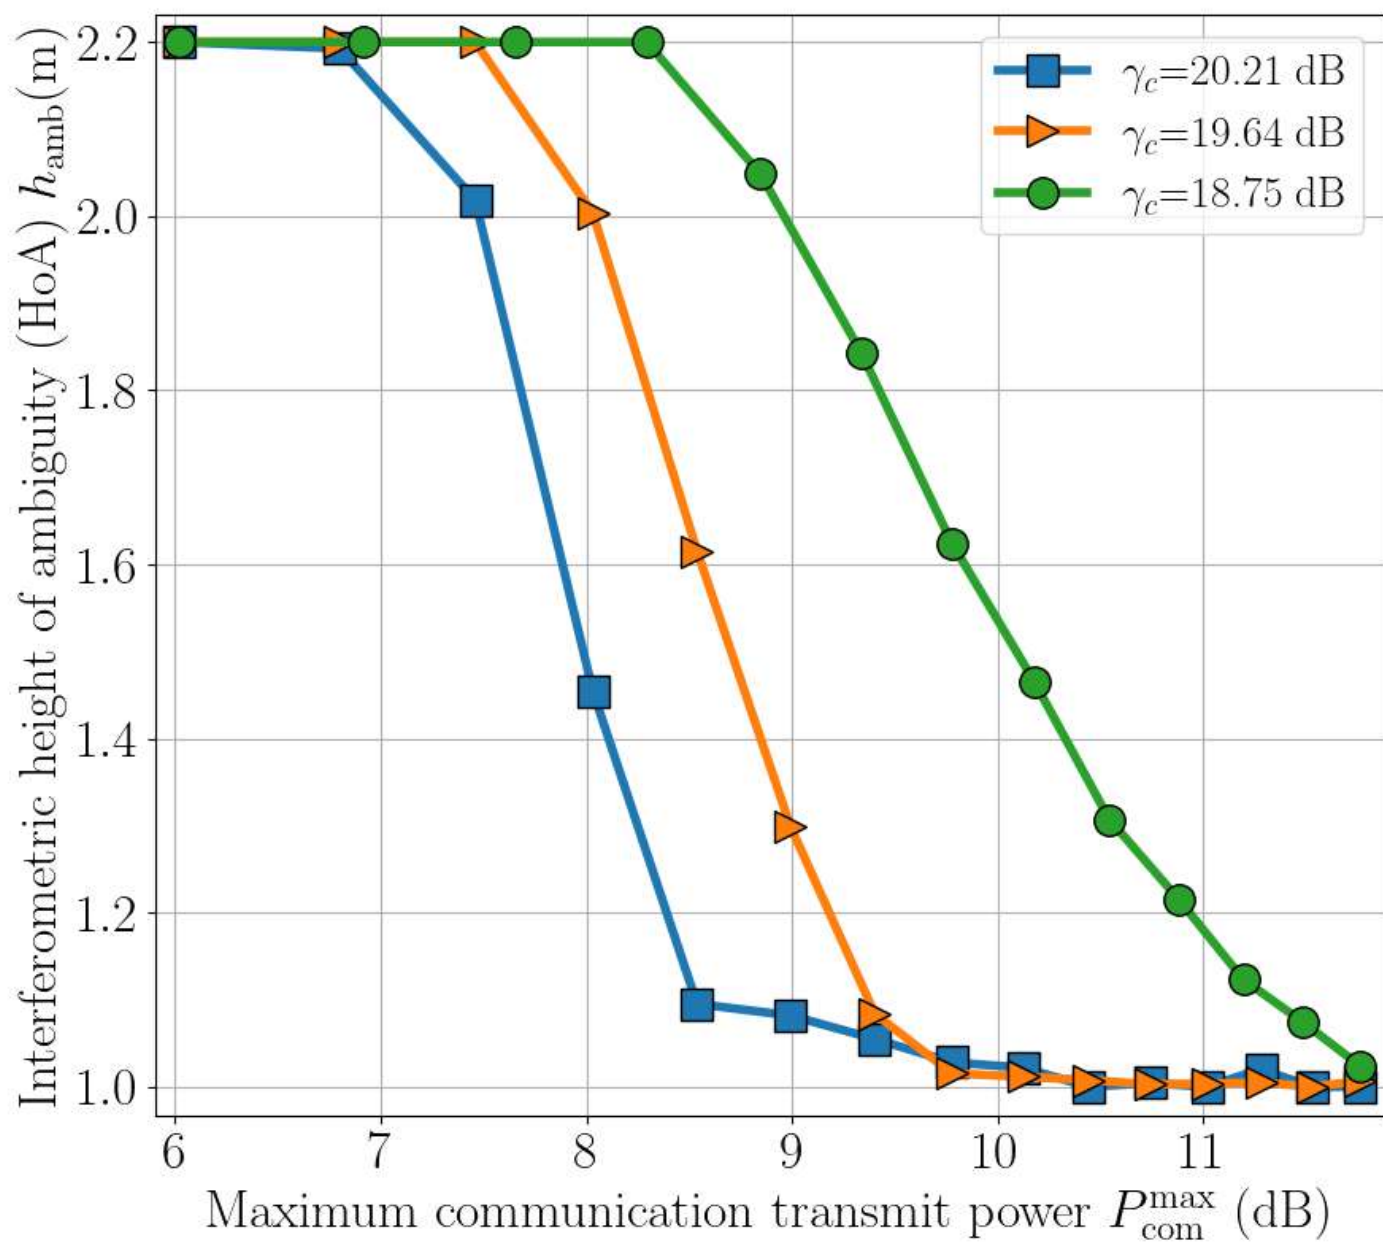

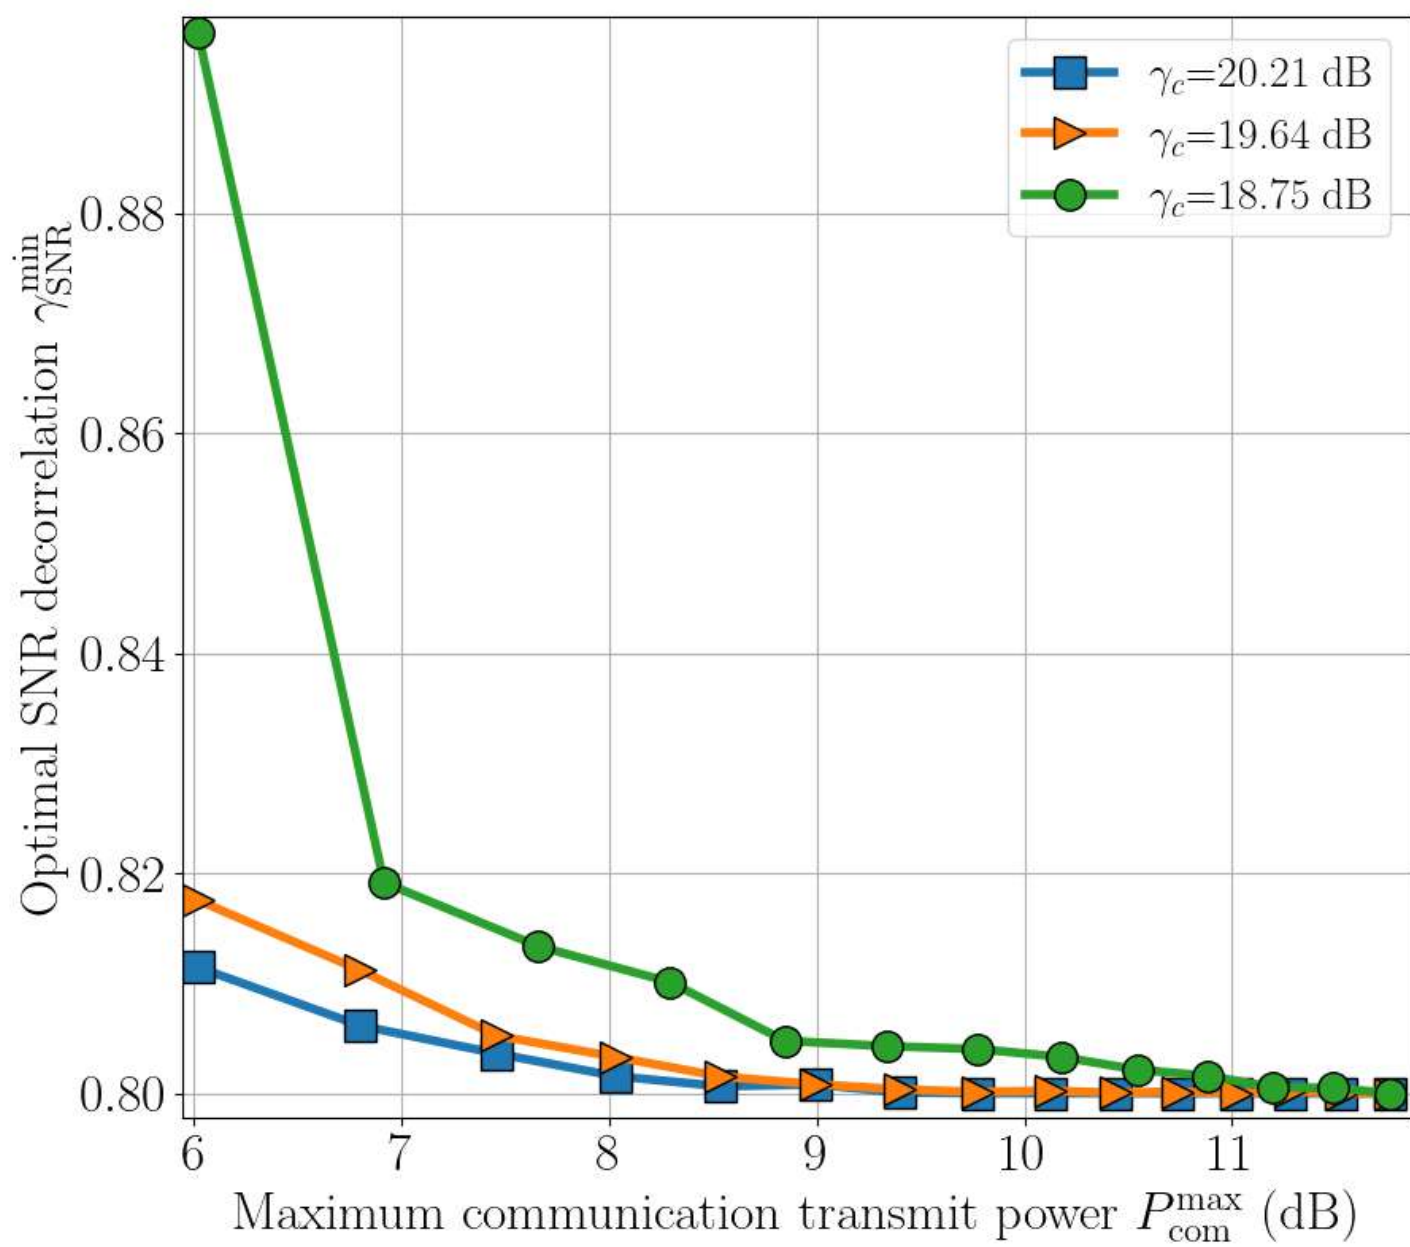

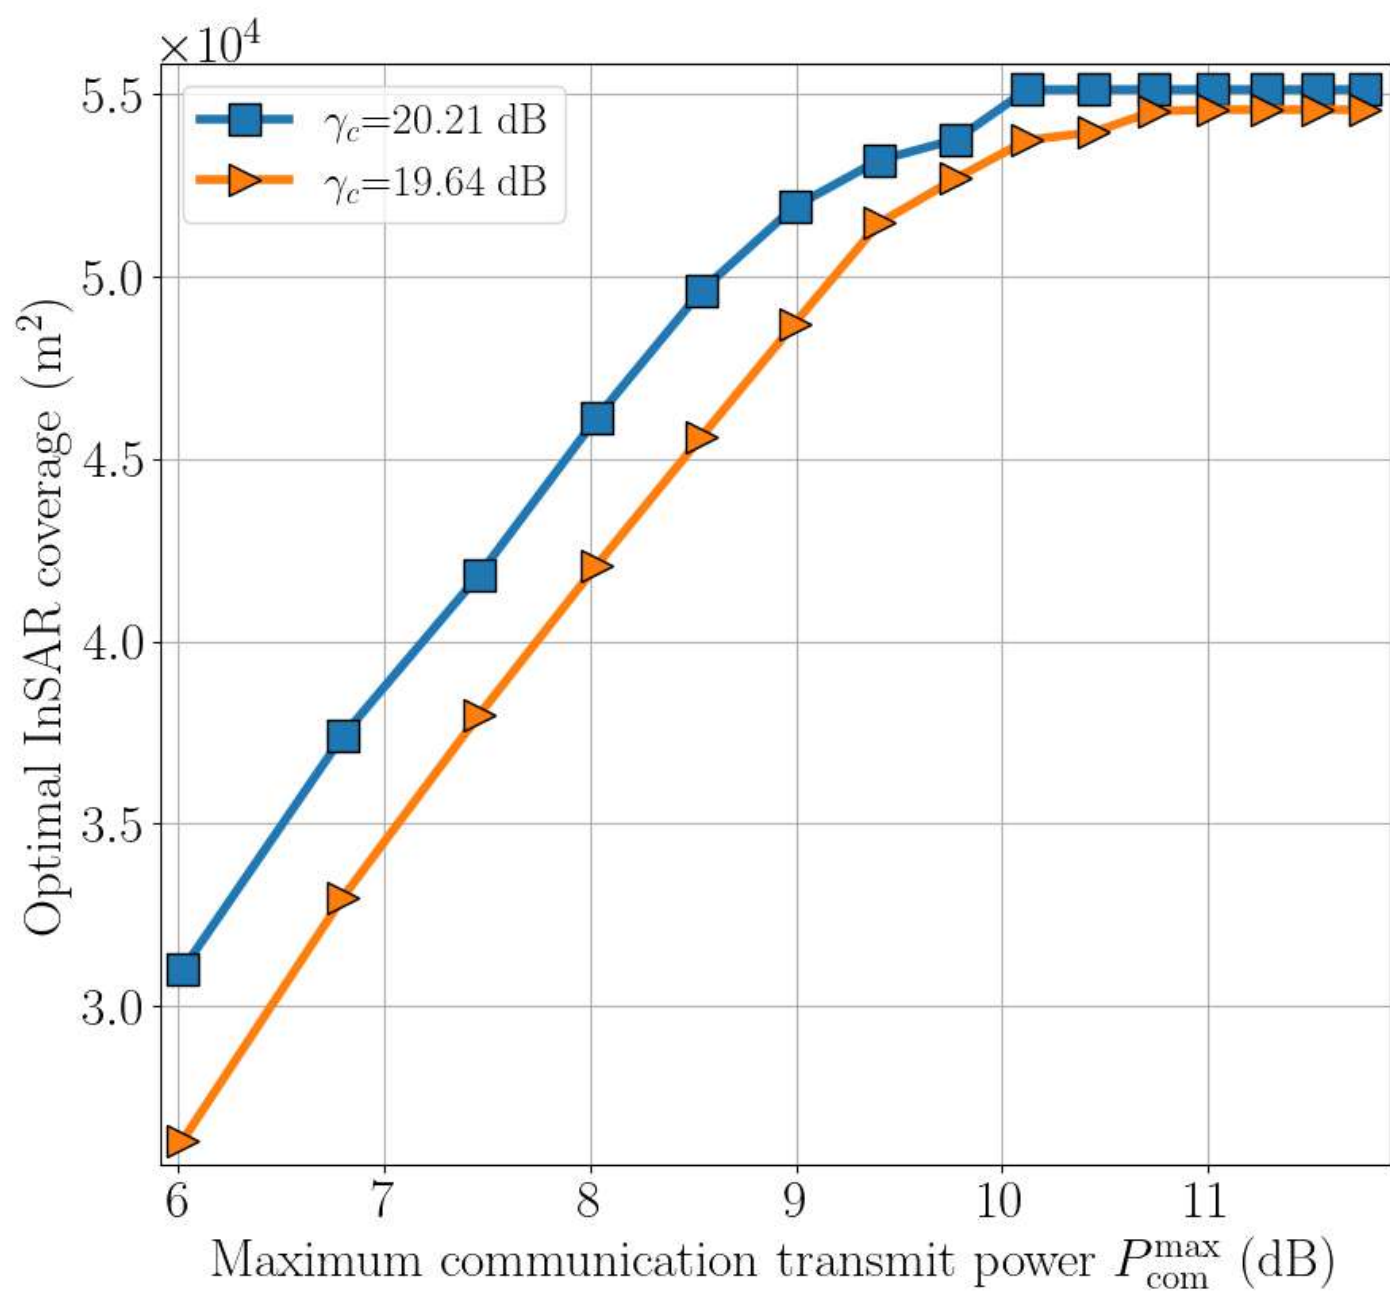

Supplement: Supplementary file 1 [file Additional_figures.pdf]
